# Supplementary material for: Belief Miner: A Methodology for Discovering Causal Beliefs and Causal Illusions from General Populations
Source: arXiv:2401.08020 source file (2024-01-16)
Supplement: Supplementary file 1 [file supplemetal_for_final_interface.tex]

\section{Re-designed and Final interface}
\label{sec:survey2}

% iterative design process. 
% Summarize the design goals. 
% 1. Make people think about climate change. (broader design goals)
%5.2 initial interface. 

% Section 6: Study 1
% Result: Learning,  selection bias, word2vec, more time
%Section 7: Revised interface
%Section 8: Experiment 
%section 9: Result

%although our design is unbiased, focusing on the variable will prompt 
 In pursuit of improved data quality, participant engagement, and overall efficiency, we embarked on a redesign process for Study 2. While our primary objective remained the same - to develop an interactive causal data collection tool for creating, modifying, and evaluating causal networks - we had two specific goals in mind. Firstly, we aimed to eliminate any potential selection bias that may have influenced participant responses. Secondly, we sought to streamline the data collection process by reducing the number of micro-tasks required. By addressing these objectives, we aimed to enhance the overall effectiveness and user experience of the interface in Study 2.  

% To achieve this, we follow several design principles. We discuss the design principles in Section \ref{subsec:design}. We build the survey interface using the \textit{Causal Attributes} as an input. We discuss the methods for processing the raw data and generating the causal attributes in Section \ref{subsec:causal_attribute}. Leveraging the design principles, we develop several modules of the collection interface. We present these modules in Section \ref{subsec:interface_modules}.

\begin{figure}
    \centering
    \includegraphics[width=0.95\textwidth]{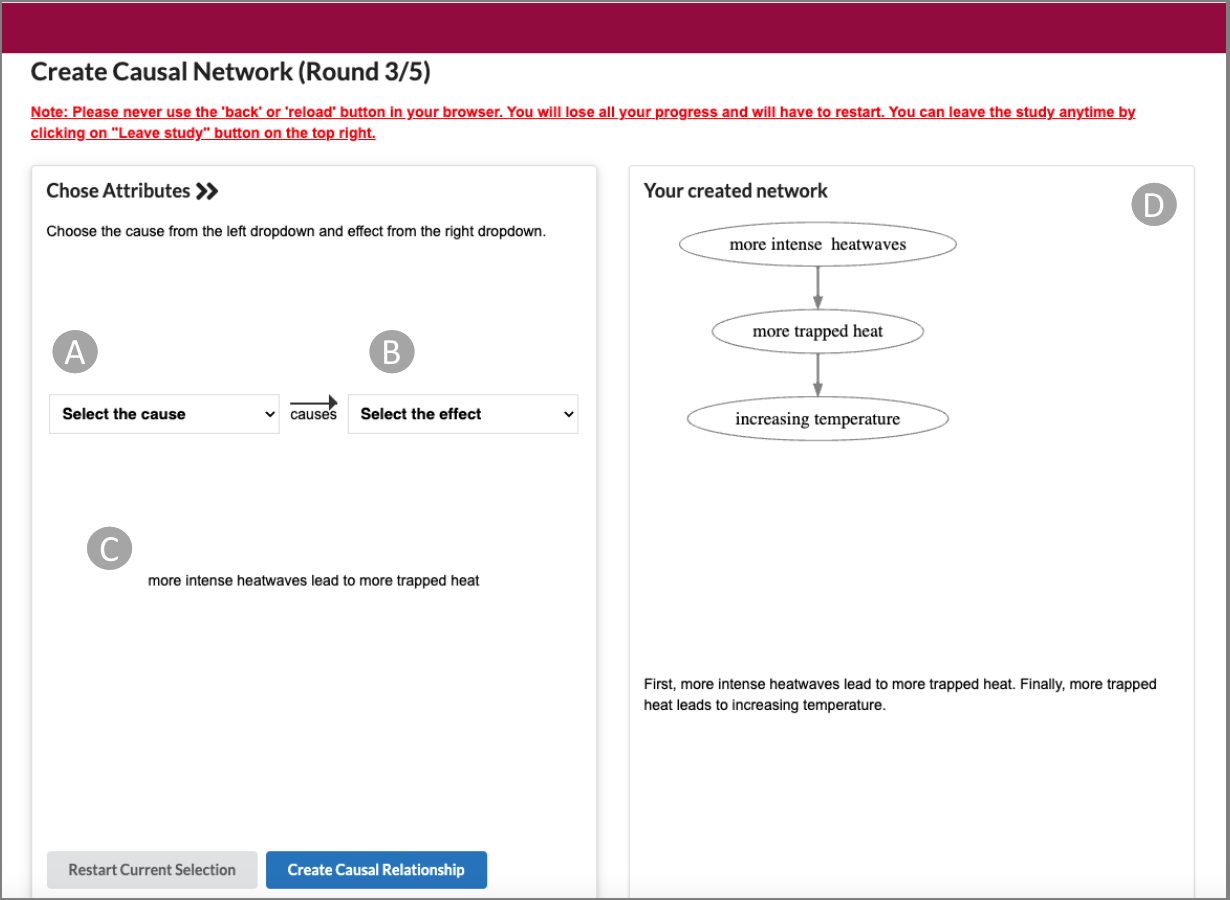}
    \caption{\textbf{Overview of the redesigned collection interface}. This example shows a causal network is being created. A shows the "cause" drop-down and B shows the "effect" drop-down. C shows the most recently created causal link as text. D contains the emerging causal network along with its textual narrative.}
    \Description{Figure \ref{fig:collection_interface_2} shows a screenshot of the collection interface. It shows a case where a crowd worker is in the process of making a causal network.}
    \label{fig:collection_interface_2}
\end{figure}

\subsection{Collection Interface Modules}\label{subsec:interface_modules}
The collection interface utilized web-based technology, employing Python as the back-end language and D3 GraphViz library for visualization \cite{bostock2011d3, d3-graphviz}. The results were stored in a MongoDB database. In order to maintain focus on wildfire-related attributes and based on the low number of votes it received in Study 1, we made the decision to exclude the attribute "renewable energy" from our input dataset, which led us to have 16 attributes with trend terms (32 attributes in total).

We describe the visual component of the several interface modules in the following sections. The modules are independent and can be implemented according to the intended sequential workflow. Snapshots of each module will be provided as supplemental material. We further describe our workflow specific to the study setup later in Section~\ref{sec:experiment2}.

\subsubsection{Instructions and Overview Module}
\label{instruction}
% \begin{figure}
%     \centering
%     \includegraphics[width=\textwidth]{figures/overview-module.pdf}
%     \caption{Instruction and Overview Module of the survey interface showing an example of the instructions page.}
%     \label{fig:overview_module}
% \end{figure}
According to DG1, the initial module in the workflow is the Instructions and Overview Module, which serves as a comprehensive guide to the entire interface. This module offers step-by-step instructions, providing an explanation of each step's purpose and functionality. Additionally, it includes visual representations of the interface pages that participants will encounter throughout their workflow, aiding in their familiarity with the interface. To assess participants' understanding, a sample task is included at the end of the module, allowing them to retry and enhance their comprehension of the overview and the concept of causality. A screenshot of this module is provided in the supplemental material for reference.

\subsubsection{Demographics And Climate Change Awareness Survey Module}
\label{demographics}
% \begin{figure}
%     \centering
%     \includegraphics[width=\textwidth]{figures/demographics.pdf}
%     \caption{Demographics Survey of the survey interface. (A) shows an example of a knowledge related question, (B) shows an example of a demographics question.}
%     \label{fig:survey}
% \end{figure}
The purpose of this module is to gather data on demographics and climate change awareness among individuals. Initially, participants are asked to respond to eight demographic questions. These questions draw inspiration from the work of \cite{snapsurveys}. It is important to note that participants have the option to withhold their personal information when answering these demographic questions.

Following the demographic section, participants are presented with four questions aimed at gauging their personal perspectives on climate change. These questions are adapted from the Six Americas Super Short Survey (SASSY) \cite{sassy}, which enables the classification of individuals into six distinct categories representing different levels of awareness regarding climate change. They categories are: Alarmed, Concerned, Cautious, Disengaged, Doubtful and Dismissive. By comparing participants' responses to national averages, we gain insights into their climate change awareness levels. We provide the demographics questions as supplemental material.

% \begin{figure}
%     \centering
%     \includegraphics[width=0.8\textwidth]{figures/creation.pdf}
%     \caption{Causal Network Creation Module of the survey interface. (A) marks the network creation
% space of the module, (C) marks the situation where two nodes are selected, (B) shows the step-by-step
% instruction box, (D) shows the available options for selecting trends for a specific attribute, (E) shows the created
% causal link in the space and (F) shows the three options for creating the causal link.}
%     \label{fig:creation_module}
% \end{figure}

\subsubsection{Causal Network Creation Module}
\label{creation}

The Causal Network Creation Module (see Figure \ref{fig:collection_interface_2}) allows participants to construct a small causal network by establishing causal relationships between attribute pairs. The use of lists or menus in the interface offers efficient scanning capabilities, predictable navigation, and quick interactions~\cite{accot1997beyond, cockburn2007predictive}. Lists enable faster information retrieval, reduce cognitive load, and can handle large amounts of content without significant performance issues. 

% However, as the list size grows, users may encounter difficulties in locating specific items or experience slower scanning speeds. To address this, design considerations such as pagination or filtering options can be implemented to maintain usability and mitigate the impact of longer lists.

The causal network creation module in our current implementation presents attributes in a randomized order to each participant to avoid selection bias and maximize exploration of the possible aggregated network. The process of creating each causal link consists of two micro-tasks: selecting an attribute as the "cause" and another attribute as the "effect," each accompanied by its corresponding trend. We refer to the completion of these two micro-tasks as a "round". In contrast to the initial interface, the redesigned interface simplifies the process of creating a causal link to just 5 clicks: two clicks to select attributes from drop-down lists and one click to confirm their choice. This simplified interaction flow eliminates the need for excessive mouse movement and reduces cognitive load, enabling participants to create causal links more efficiently and with fewer actions~\cite{cockburn2007predictive}. Participants engage in multiple rounds to construct a small causal network, with the current interface implementation allowing for the creation of one network per session. During each round, participants have the option to restart their choices as many times as they desire. A detailed workflow of the module is described in Section \ref{sec:experiment2}.
 
We represent the creation of a causal relation through the drawing of links between nodes and describing the causal relationships using natural language text. Following the approach of \cite{berenberg2018efficient}, we maintain a narrative flow within the causal network. Consequently, after the first round, participants are required to establish a causal link between a previously chosen attribute and a new attribute. To facilitate this, in rounds two and onward, the drop-down menus are populated with the attributes selected in previous rounds. When participants choose an attribute as the cause or effect, the remaining available new attributes are populated in the opposite drop-down menu. Throughout the process of constructing the network, participants can view their previously created links and receive information on the remaining rounds, providing a sense of progress.

\begin{figure}
    \centering
    \includegraphics[width=0.95\textwidth]{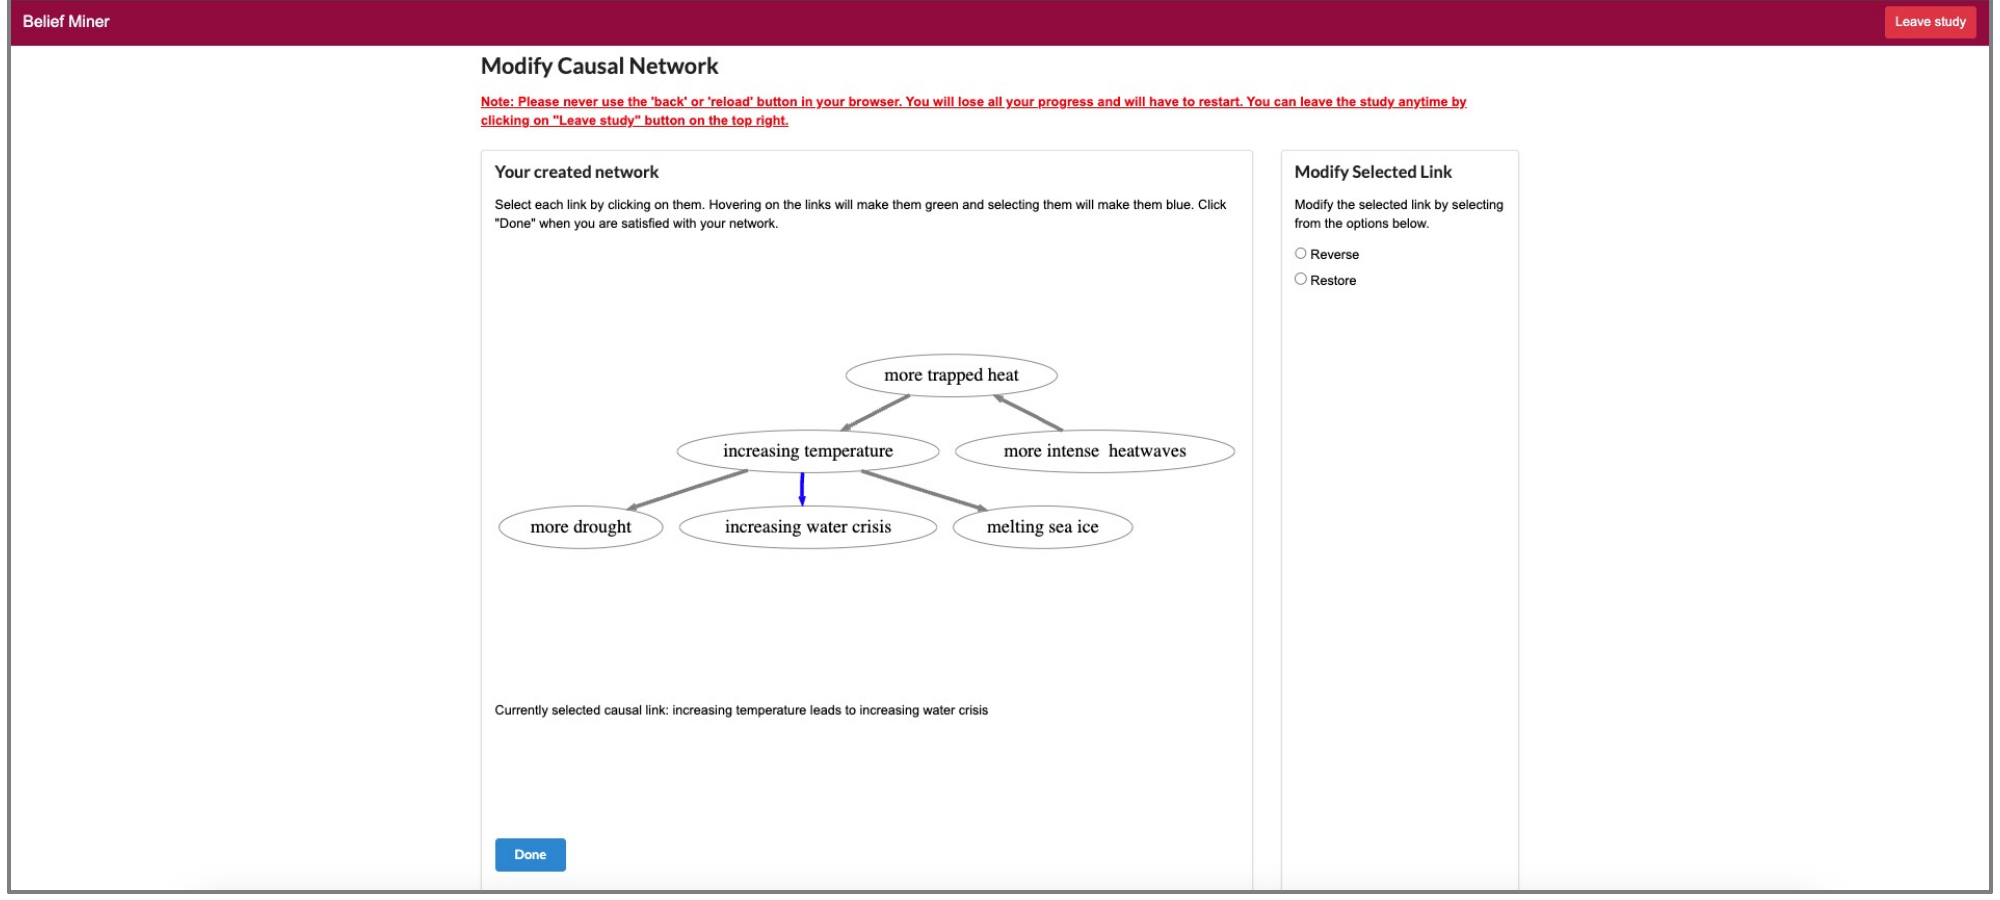}
    \caption{\textbf{Causal Network Alteration Module of the survey interface.} The link marked in \textcolor{blue}{blue} is the link currently selected for alteration. The box on the right provides available alteration options.}
    \Description{Figure \ref{fig:alteration_2} shows the screenshot of the \textit{Causal Network Alteration Module}. It shows a phase where a crowd worker modifies one network link.}
    \label{fig:alteration_2}
\end{figure}

\subsubsection{Causal Network Alteration Module}
\label{alternation}

In accordance with \textit{DG2}, we have developed the Causal Network Alteration Module to enable participants to modify the network they have created by altering each network link (see Figure \ref{fig:alteration_2}). The module provides participants with the option to change the originally selected link direction.
%the users create a causal network.

\begin{figure}
    \centering
    \includegraphics[width=\textwidth]{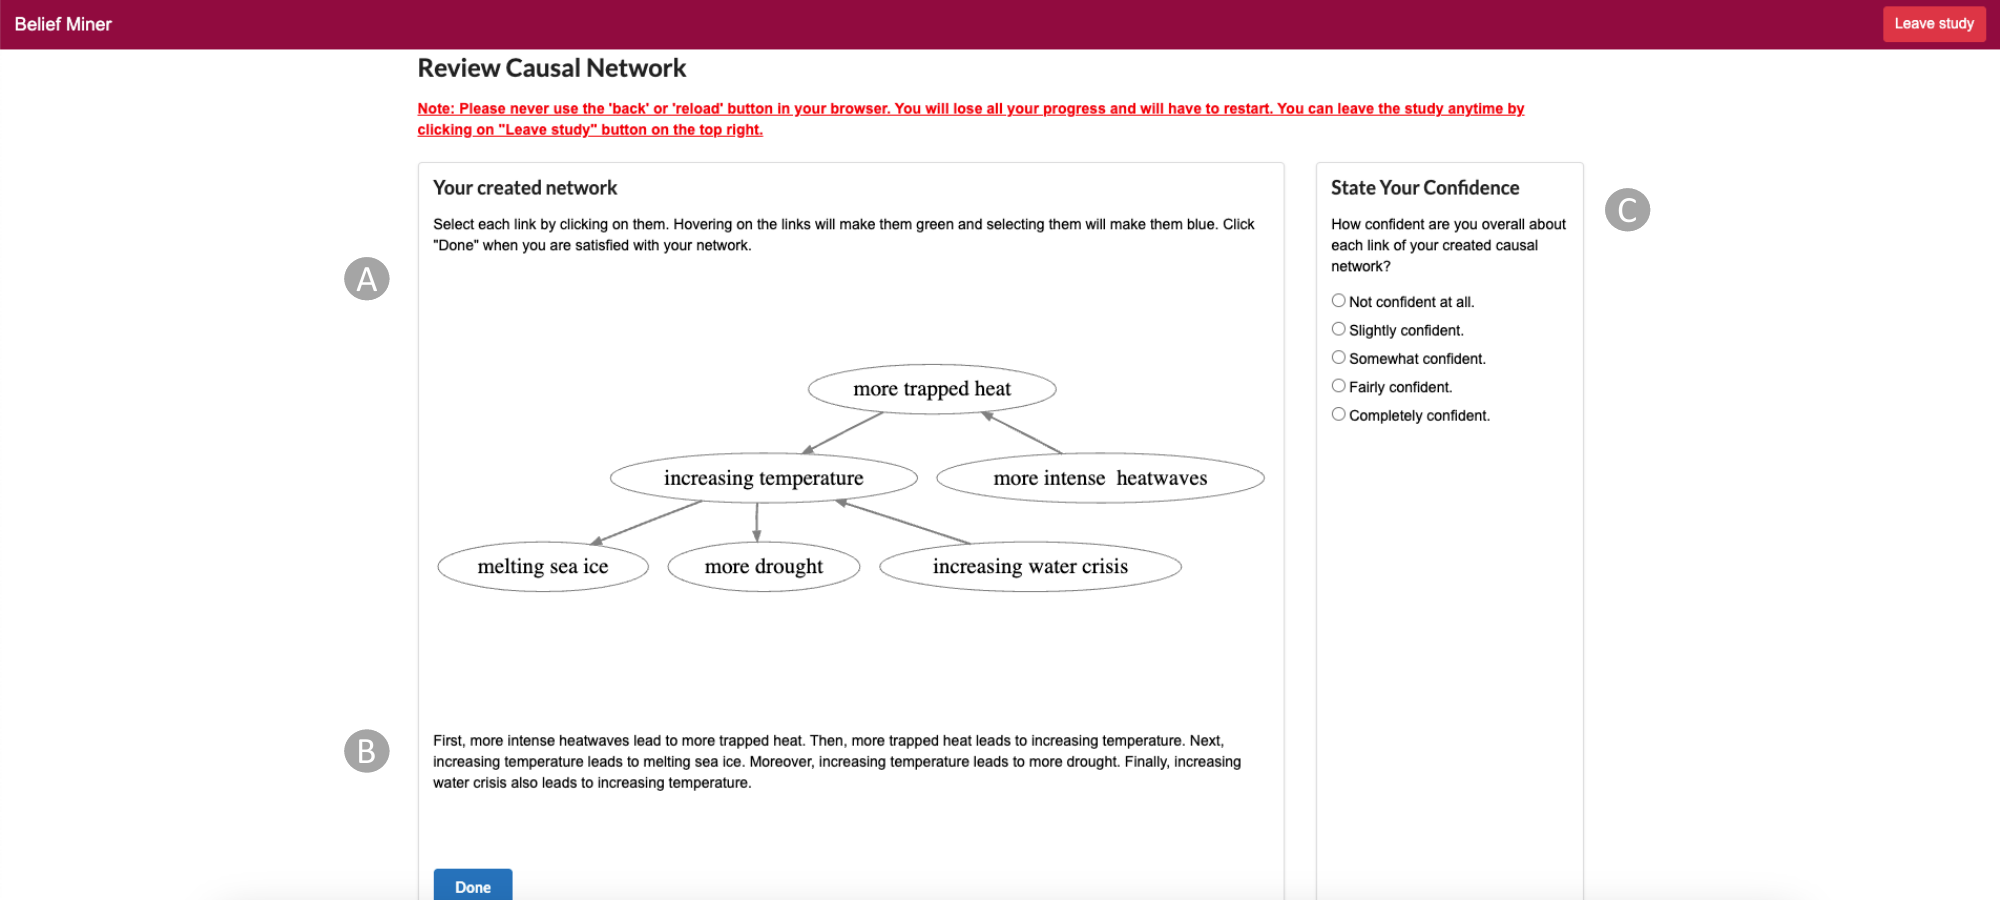}
    \caption{
    \textbf{Causal Network Interpretation and Evaluation Module of the survey interface.} (A) shows the final network after alteration, (B) shows the natural language text for reading the created network and (C) marks the options for evaluating the created network as a range of confidence levels.}
    \Description{Figure \ref{fig:graph_eval_2} shows the screenshot of the \textit{Causal Network Interpretation and Evaluation Module} of the interface. It shows a phase where a crowd worker looks at the created network and evaluates it.}
    \label{fig:graph_eval_2}
\end{figure}

\subsubsection{Causal Network Interpretation and Evaluation Module}
\label{interpretation}

In this final step, participants are asked to evaluate the causal network they have created (and potentially altered)(see Figure \ref{fig:graph_eval_2}). Consistent with \textit{DG3}, we provide participants with the natural language text representation of their created network, which serves as a narration of the network. To generate this text, we utilize a combination of a graph traversal algorithm and a simple text template to translate the network into a textual narrative.

Subsequently, participants are given the opportunity to evaluate their created network. The evaluation is collected by assessing their confidence level using a 5-point Likert scale. This module always follows the completion of the \textit{Causal Network Alteration Module}.
\subsubsection{Interface Evaluation Module}
\label{evaluation_interface}
% \begin{figure}
%     \centering
%     \includegraphics[width=\textwidth]{figures/interface_evaluation.pdf}
%     \caption{Interface Evaluation Module of the survey interface.}
%     \label{fig:interface_evaluation}
% \end{figure}

The purpose of this module is to allow participants to evaluate the overall usability and knowledge gained from the data collection interface. Drawing inspiration from the System Usability Scale (SUS) \cite{sus}, participants are presented with a series of seven statements. Five of these statements are related to usability, while the remaining two focus on knowledge acquisition.

To measure usability, participants are provided with both positive and negative statements, which are presented in alternating order. These statements assess participants' perception of the interface's usability and its effectiveness in achieving their goals. The knowledge-related statements aim to evaluate the impact of creating a causal network on participants' original perceptions and understanding of the topic.

A detailed description of the seven statements can be found in Section \ref{sec:usability_statements}.

}

We mention the sequential workflow of the crowd workers below:
 \begin{enumerate}
      \item \textbf{Read the instructions and perform and pass the test.} These tasks were performed in the \textit{Instructions and Overview Module} (Section~\ref{instruction}). Each crowd worker reads an overview of the whole interface as a step-by-step guide, along with the explanation and purpose of each step. They have the opportunity to go back to previous pages or restart anytime. They can refer to the pictures of the interface in different phases of their upcoming workflow that are provided in the module. Next, they encounter a simple instance of building a causal relation between two attributes. If they can pass this test, they proceed to the next step. If they fail this test, they can always restart this module and retry this test to improve their understanding.
     \item \textbf{Complete the demographics survey.} This task was performed in the \textit{Demographics and Climate Change Awareness Survey Module} (Section~\ref{demographics}). Each crowd worker answers 8 questions regarding their demographics, ad 4 questions on climate change awareness. The demographics questions are about their ethnicity, gender, marital status, geographical location (state and county), education, employment status, and age group. In each demographic question, they have an option not to provide their information. We provide the demographics questions in the supplemental materials.
     \item\textbf{Create a causal network.} This task was performed in the \textit{Causal Network Creation Module} (Section~\ref{creation}). Each crowd worker will create five different causal links to build a small causal network. They need to perform two micro-tasks to create each causal link.
\begin{itemize}
    \item Choose the "cause" (and its respective trend) from the cause drop-down. 
    \item Choose the "effect" (and its respective trend) from the effect drop-down.
\end{itemize} 
    The crowd workers are free to choose the attributes and their trends based on their personal perceptions. For example, they may choose the attribute ``CO2'' with an ``increasing'' or ``decreasing'' trend. Performing these two microtasks will automatically create a causal relationship. Say, for the chosen two trended attributes, \textit{increasing emissions} as the "cause" and \textit{increasing CO2} as the "effect", the created causal relation would be \textit{increasing emissions} leads to \textit{increasing CO2}. 

After the first link, the workers are asked to select a new node that has not been selected before and an already selected node in order to create a new causal relation, adding to the emerging small network. 
     \item\textbf{Alter causal network. }This task is performed in the \textit{Causal Network Alteration Module} (Section~\ref{alternation}). Each crowd worker can alter their created causal network from the previous step by choosing the link they want to change by left-clicking on it and
selecting from the available options for alteration. The options are: \textit{change direction} and \textit{do not modify anything}. 
     \item\textbf{Evaluate causal network.} This task is performed in the \textit{Causal Network Interpretation and Evaluation Module} (Section~\ref{interpretation}). Each crowd worker can read their causal network and view it in a node-link diagram or Directed Acyclic Graph (DAG) format. On a scale of 1 to 5, they also provide their confidence level to the created networks.
     
     \item \textbf{Evaluate the interface}. After creating a causal network, each crowd worker is asked to evaluate the interface based on seven usability and learning statements on a 5-point Likert Scale using the \textit{Interface Evaluation Module} (Section~\ref{evaluation_interface}). 
     
    %  Here each participant has to evaluate the survey interface. They are provided five usability-related and two knowledge-related statements and have to choose their level of agreement.  
     
     \item \textbf{Verification and compensation}. Each crowd worker is provided with a unique code at the end of their participation (on AMT) or redirected to a specific link (on Prolific). We used these mechanisms to validate the results, discard any incomplete data, and compensate the crowd worker. 
 \end{enumerate}
